# Supplementary material for: Reducing Redundant Work in Jump Point Search
Source: arXiv:2306.15928 source file (2023-06-28)
Supplement: Supplementary file 1 [file main.tex]

%File: anonymous-submission-latex-2023.tex
\documentclass[a4paper]{article} % DO NOT CHANGE THIS
\usepackage{graphicx} % DO NOT CHANGE THIS
% \urlstyle{rm} % DO NOT CHANGE THIS
% \def\UrlFont{\rm}  % DO NOT CHANGE THIS
\usepackage{natbib}  % DO NOT CHANGE THIS AND DO NOT ADD ANY OPTIONS TO IT
\usepackage{caption} % DO NOT CHANGE THIS AND DO NOT ADD ANY OPTIONS TO IT
\usepackage{float}
\usepackage{geometry}
 \geometry{
 a4paper,
 total={170mm,257mm},
 left=20mm,
 top=20mm,
 }
 \usepackage{subcaption}
%
% These are recommended to typeset algorithms but not required. See the subsubsection on algorithms. Remove them if you don't have algorithms in your paper.
\usepackage[algoruled,vlined,linesnumbered]{algorithm2e}

\usepackage{array}
\usepackage{comment}
\usepackage{mathtools}
\usepackage{cleveref}
\usepackage{booktabs}
\usepackage{placeins}

\begin{document}

\section{Appendix}
\subsection{Improvement on node expansion} 
In the main paper, we show the proportion of suboptimal nodes in synthetic maps and original domain maps.
Here, we report the number of suboptimal nodes of JPS and CJPS in domain maps with dynamic changes.

Table~\ref{tb:subcnt-a} shows the comparison of total and suboptimal node expansion.
We can see that CJPS reduces more than half of suboptimal node expansion (\emph{sub}), but there are still 20\% left and most of them are from suboptimal parents,
which can be improved in future work.

\begin{table}[H]
  \begin{subtable}{\linewidth}
  \centering
  \centering
\begin{tabular}{lrrrrrr}
  \toprule
  domain    & \#maps & mean & median & sub\% & subp\% \\
  \midrule
  dao       & 154 & 215  & 62   & 30  & 64  \\
  bgmaps    & 75  & 98   & 41   & 27  & 65  \\
  starcraft & 75  & 1038 & 777  & 28  & 73  \\
  street    & 30  & 596  & 312  & 33  & 84  \\
  iron      & 35  & 5065 & 3962 & 43  & 88  \\
  maze512   &  6  & 8863 & 2516 &  0  & --- \\
  random10  &  1  & 7574 & 7527 & 33  & 18 \\
  rooms     &  4  & 1766 &  653 & 25  & 26 \\
  \bottomrule
\end{tabular}

  \caption{}
  \label{tb:subcnt-a}
  \end{subtable}
  \begin{subtable}{\linewidth}
  \centering
  \begin{tabular}{rrrrrrrrr}
\toprule
other domains & alg  & avg/query     & median/query & total   & sub    & propagated & sub\% & subp\% \\
\midrule
maze512       & cjps & 4341.64 & 1285.5 & 2604981 & 2833   & 1265       & 0.01 & 44.6  \\
              & jps  & 4368.02 & 1298.0 & 2620810 & 18668  & 1813       & 0.07 & 9.7  \\ \hline
rooms         & cjps & 1960.19 & 907.5  & 784075  & 179596 & 38068      & 22.9 & 21.1  \\
              & jps  & 2028.12 & 942.0  & 811249  & 206770 & 52413      & 25.4 & 25.3  \\
\bottomrule
\end{tabular}

  \caption{}
  \label{tb:subcnt-b}
  \end{subtable}
  \caption{Node expansion statistic when r=0.1\%, where \emph{avg} and \emph{median} are for queries, which represent difficulty. 
  \emph{total, sub} and \emph{propagated} are cumulated from all queries, \emph{sub\%}=$\frac{sub}{total}$, \emph{subp\%}=$\frac{propagated}{sub}$.}
  \label{tb:subcnt}
\end{table}

\subsection{Improvement on various density of obstacles}
Figure~\ref{fig:domain-dist} shows the query speed-up distribution for r $\in$ \{0, 0.1, 0.5, 1, 1.5\}\%.
We can see that the speed-up median (the black bar in the box) increases till some points, then drops, which can be explained by the discussion in \emph{Exp-1} from the main paper.
\begin{figure}[H]
  \centering
  \includegraphics[width=1\linewidth]{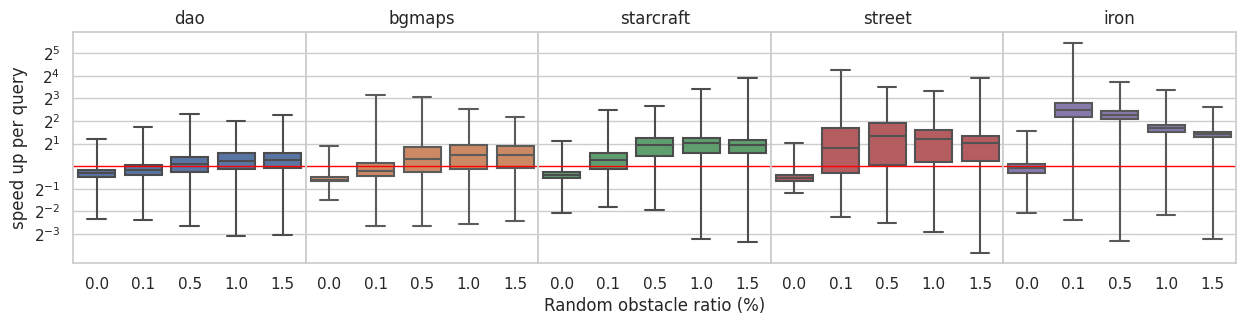}
  \caption{Query speed-up distribution, the red line is 1, above it means CJPS is faster.}
  \label{fig:domain-dist}
\end{figure}

\subsection{Improvement on other domains}
The results of three sets of maps are not presented in the main paper, but worth mention:
\begin{itemize}
  \item low resolution \emph{street}: scaled down the resolution from 1024 to 512, 256;
  \item \emph{maze512}: 6 maps in size 512$\times$512, the difference is corridor width \emph{W} $\in$ \{1, 2, 4, 8, 16, 32\};
  \item \emph{rooms}: 4 maps in size 512$\times$512, the map is composed of multiple rooms with the same size \emph{L} $\in$ \{8, 16, 32, 64\}, and each room has 4 adjacent reachable/not-reachable rooms.
\end{itemize}

Figure~\ref{fig:other-dist} shows the result. 
In \emph{street}, CJPS is less effective on lower resolution maps as less scanning cost and jump points in search space. 
In both \emph{maze512} and \emph{rooms}, JPS terminates the diagonal recursion early due to the topology of maps, see in Table~\ref{tb:subcnt-b}.
Thus, there is not much redundant work to prune for CJPS, and it only has the advantage when the \emph{W} or \emph{L} is large.

\begin{figure}[H]
    \begin{subfigure}{.5\textwidth}
    \centering
    \includegraphics[width=\textwidth]{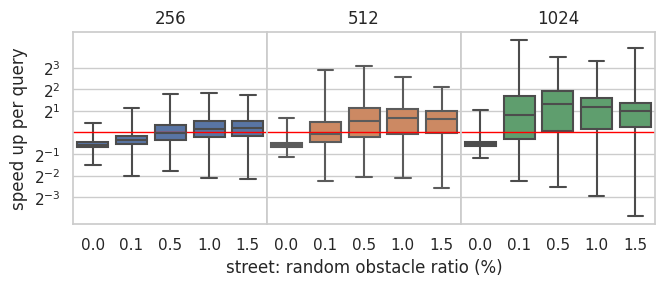}
    \end{subfigure}%
    \begin{subfigure}{.5\textwidth}
    \centering
    \includegraphics[width=\textwidth]{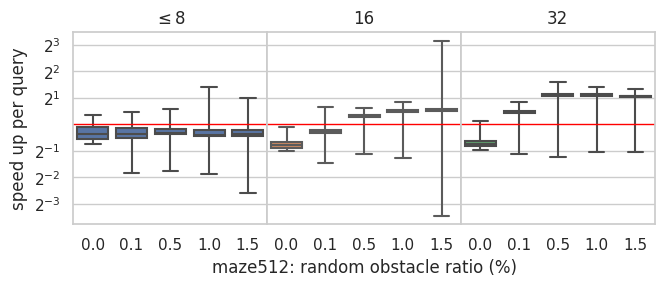}
    \end{subfigure}

    \begin{subfigure}{.5\textwidth}
    \centering
    \includegraphics[width=\textwidth]{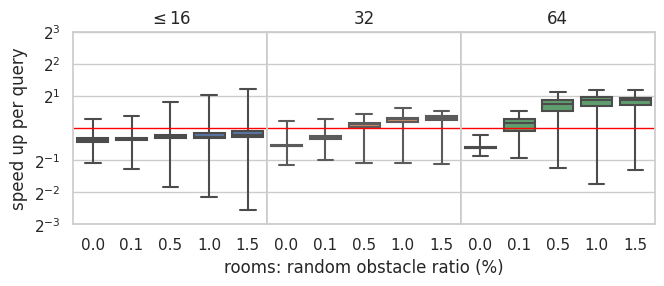}
    \end{subfigure}%
    \begin{subfigure}{.5\textwidth}
    \hspace{-5mm}
    \vspace{6mm}
    \centering
    \includegraphics[width=.6\textwidth]{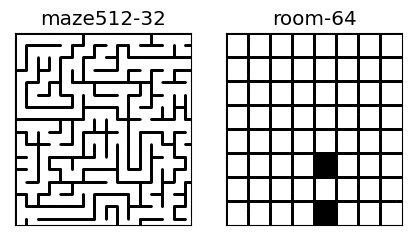}
    \end{subfigure}
    \caption{Query speed-up distribution of domains: \emph{street}, \emph{maze512}, \emph{rooms}, bottom right shows maps from maze and room.}
    \label{fig:other-dist}
\end{figure}
\end{document}
