# Supplementary material for: Reducing Redundant Work in Jump Point Search
Source: arXiv:2306.15928 source file (2023-06-28)
Supplement: Supplementary file 2 [file subcnt-2.tex]

\begin{tabular}{rrrrrrrrr}
\toprule
other domains & alg  & avg/query     & median/query & total   & sub    & propagated & sub\% & subp\% \\
\midrule
maze512       & cjps & 4341.64 & 1285.5 & 2604981 & 2833   & 1265       & 0.01 & 44.6  \\
              & jps  & 4368.02 & 1298.0 & 2620810 & 18668  & 1813       & 0.07 & 9.7  \\ \hline
rooms         & cjps & 1960.19 & 907.5  & 784075  & 179596 & 38068      & 22.9 & 21.1  \\
              & jps  & 2028.12 & 942.0  & 811249  & 206770 & 52413      & 25.4 & 25.3  \\
\bottomrule
\end{tabular}
