# Supplementary material for: Reducing Redundant Work in Jump Point Search
Source: arXiv:2306.15928 source file (2023-06-28)
Supplement: Supplementary file 3 [file subcnt.tex]

\begin{tabular}{llrrrrrrrrr}
\toprule
domain    & alg  & avg/query & median/query & total    & sub      & propagated & sub\% & subp\% \\
\midrule
bgmaps    & cjps & 148.04   & 94.0    & 1110307  & 182597   & 99698    & 16 & 55 \\
          & jps  & 173.25   & 110.0   & 1299410  & 377534   & 181407   & 29 & 48 \\ \hline
dao       & cjps & 218.99   & 72.0    & 3387754  & 742711   & 459622   & 22 & 62 \\
          & jps  & 247.97   & 76.0    & 3836030  & 1193101  & 711532   & 31 & 60 \\ \hline
starcraft & cjps & 1198.39  & 950.5   & 8987933  & 1635767  & 1018884  & 18 & 62 \\
          & jps  & 1461.69  & 1150.0  & 10962671 & 3617392  & 2034824  & 33 & 56 \\ \hline
street    & cjps & 318.65   & 187.0   & 1911873  & 421851   & 251884   & 22 & 60 \\
          & jps  & 364.73   & 205.0   & 2188389  & 701135   & 406462   & 32 & 58 \\ \hline
iron      & cjps & 10348.18 & 9486.5  & 36218627 & 7922502  & 3987305  & 22 & 50 \\
          & jps  & 15128.22 & 13800.5 & 52948787 & 24663218 & 10447322 & 47 & 42 \\
\bottomrule
\end{tabular}
